# Supplementary material for: LICO: Explainable Models with Language-Image Consistency
Source: arXiv:2310.09821 source file (2023-10-15)
Supplement: Supplementary file 1 [file supp_main.tex]

\documentclass{article}

% if you need to pass options to natbib, use, e.g.:
%     \PassOptionsToPackage{numbers, compress}{natbib}
% before loading neurips_2023

% ready for submission
\usepackage[final]{neurips_2023}
%\usepackage[toc,title,page]{appendix}

% to compile a preprint version, e.g., for submission to arXiv, add add the
% [preprint] option:
%     \usepackage[preprint]{neurips_2023}

% to compile a camera-ready version, add the [final] option, e.g.:
%     \usepackage[final]{neurips_2023}

% to avoid loading the natbib package, add option nonatbib:
%    \usepackage[nonatbib]{neurips_2023}

\usepackage[utf8]{inputenc} % allow utf-8 input
\usepackage[T1]{fontenc}    % use 8-bit T1 fonts
\usepackage{url}            % simple URL typesetting
\usepackage{booktabs}       % professional-quality tables
\usepackage{amsfonts}       % blackboard math symbols
\usepackage{nicefrac}       % compact symbols for 1/2, etc.
\usepackage{microtype}      % microtypography
\usepackage{xcolor}         % colors
\definecolor{citecolor}{HTML}{1F801F}
\definecolor{linkcolor}{HTML}{ED1C24}
\usepackage[breaklinks=true,colorlinks,citecolor=citecolor, linkcolor=linkcolor, bookmarks=false]{hyperref}

\usepackage{multirow}
\usepackage{bbding}

\usepackage{amsmath}
\usepackage{amssymb}
\usepackage{mathtools}
\usepackage{amsthm}

\usepackage{url}            % simple URL typesetting
\usepackage{booktabs}       % professional-quality tables
\usepackage{nicefrac}       % compact symbols for 1/2, etc.
\usepackage{microtype}      % microtypography
\usepackage{bbding}
\usepackage{graphicx}
\usepackage{color}
\usepackage{graphicx}
\usepackage{textcomp}
\usepackage{bm}
\usepackage{multirow}
\usepackage{booktabs}
\usepackage{bbding}
\usepackage{mfirstuc}
\usepackage[misc]{ifsym} 
\usepackage{graphics}
\usepackage{makecell}
\usepackage{amsthm}
\usepackage{color}
\usepackage[ruled]{algorithm2e}

\usepackage{wrapfig}
\usepackage{graphicx}

 % use \tabincell{c}{.....} to linefeed

% \newcommand{\gbf}[1]{\green{\bf{\fn{(#1)}}}}
% \newcommand{\gbf}[1]{\bf{\scriptsize{ #1}}} % footnotesize 
% \newcommand{\rbf}[1]{\red{\bf{\fn{(#1)}}}}
% \newcommand{\rbf}[1]{\bf{\scriptsize{ #1}}}

\usepackage{xspace}
 % vector
 % matrix

% \newcommand{\blue}[1]{\textcolor{blue}{#1}}
% \newcommand{\red}[1]{\textcolor{red}{#1}}
% operator in optimization

% \newtheorem{proof}[theorem]{Proof}

% \newcommand{\li}[1]{{\textcolor{red}{YY: #1}}}
% \newcommand{\lei}[1]{{\textcolor{cyan}{YM: #1}}}
% \newcommand{\longzili}[1]{{\textcolor{green}{L: #1}}}

\title{LICO: Explainable Models with Language-Image COnsistency\\
---Supplementary Materials---}

% The \author macro works with any number of authors. There are two commands
% used to separate the names and addresses of multiple authors: \And and \AND.
%
% Using \And between authors leaves it to LaTeX to determine where to break the
% lines. Using \AND forces a line break at that point. So, if LaTeX puts 3 of 4
% authors names on the first line, and the last on the second line, try using
% \AND instead of \And before the third author name.

\author{Paper ID: 6636}

% \author{
% *%
%   % examples of more authors
%   % \And
%   % Coauthor \\
%   % Affiliation \\
%   % Address \\
%   % \texttt{email} \\
%   % \AND
%   % Coauthor \\
%   % Affiliation \\
%   % Address \\
%   % \texttt{email} \\
%   % \And
%   % Coauthor \\
%   % Affiliation \\
%   % Address \\
%   % \texttt{email} \\
%   % \And
%   % Coauthor \\
%   % Affiliation \\
%   % Address \\
%   % \texttt{email} \\
% }

\begin{document}

\maketitle

% \input{abstract}
%\begin{appendices}

\input{A}
\input{C}
\input{B}

% \newpage

%\end{appendices}

% \bibliographystyle{neurips_2023}
% \bibliography{neurips_2023}
% \bibliographystyle{unsrt}
% \bibliography{neurips_2023}
% {
% \small

%%%%%%%%%%%%%%%%%%%%%%%%%%%%%%%%%%%%%%%%%%%%%%%%%%%%%%%%%%%%

\end{document}
